# Supplementary material for: A Large Hadron Electron Collider at CERN: Report on the Physics and Design Concepts for Machine and Detector
Source: arXiv:1206.2913 source file (2012-09-07)
Supplement: Supplementary file 1 [file appendix1.tex]

\section*{Tasks for a Technical Design Report}
\section*{Building and Operating the LHeC}
